# Supplementary material for: Optimal Electrical Oblivious Routing on Expanders
Source: arXiv:2406.07252 source file (2024-06-11)
Supplement: Supplementary file 1 [file appendix.tex]

\section{Appendix}

\subsection{Proof of Lemma \ref{lemma_norm_preserved_random_cut}}

To prove the lemma, we first rewrite the expected \(\ell_1\)-norm of the cut:
\begin{align*}
	\mathbb{E}\left[ \matr{W} \matr{B}^\trp \matr{1}_{S_{\geq t}} \right] & = \mathbb{E}\left[ \sum_{(a, b) \in E}{w(a, b) \cdot \left\lvert \matr{1}_{S_{\geq t}}(a) - \matr{1}_{S_{\geq t}}(b) \right\rvert} \right] \\
	& = \sum_{(a, b) \in E}{w(a, b) \cdot \mathbb{E}\left[\left\lvert \matr{1}_{S_{\geq t}}(a) - \matr{1}_{S_{\geq t}}(b) \right\rvert\right]}  \\
	& = \sum_{(a, b) \in E}{w(a, b) \cdot \mathbbm{1}_{\left\lvert \matr{1}_{S_{\geq t}}(a) - \matr{1}_{S_{\geq t}}(b) \right\rvert = 1}}  \\
	& = \sum_{(a, b) \in E}{w(a, b) \cdot \mathbb{P}\left[\left\lvert \matr{1}_{S_{\geq t}}(a) - \matr{1}_{S_{\geq t}}(b) \right\rvert = 1\right]}  \\
	& = \sum_{(a, b) \in E}{w(a, b) \cdot \mathbb{P}\left[ \min\{\matr{x}(a), \matr{x}(b)\} \leq t < \max\{\matr{x}(a), \matr{x}(b)\} \right]}.
\end{align*}
The last equality arises from the definition of the set \(S_{\geq t}\) and the fact that \(\matr{x} \in [0, 1]^V\). Using our assumption about the uniform distribution of \(t\) in the interval \([0, 1]\), we obtain the desired result:
\begin{align*}
\mathbb{E}\left[ \matr{W} \matr{B}^\trp \matr{1}_{S_{\geq t}} \right] & =  \sum_{(a, b) \in E}{w(a, b) \cdot \mathbb{P}\left[ \min\{\matr{x}(a), \matr{x}(b)\} \leq t < \max\{\matr{x}(a), \matr{x}(b)\} \right]} \\
& = \sum_{(a, b) \in E}{w(a, b) \cdot \left\lvert \matr{x}(a) - \matr{x}(b)
 \right\rvert} \\
 & = \left\lVert \matr{W} \matr{B}^\trp \matr{x} \right\rVert_1.
\end{align*}

\subsection{Proof of Lemma \ref{lemma_program_minimizer_continuous}}
We prove this lemma by showing that from any \(\matr{z} \in \R^F\) we can construct \(\matr{z}' \in [0, 1]^F\), such that the value for \(\matr{z}'\) of the given program is less or equal to the one for \(\matr{z}\). Therefore, there will always exist a minimizer of the program that lies in \([0, 1]^F\).

Thus, for a fixed \(\matr{x} \in [0, 1]^C\), let \(\matr{z} \in \R^F\) be arbitrary and construct \(\matr{z}'\) by ``capping'' all elements of \(\matr{z}\) below \(0\) with a \(0\) in that respective entry, and all elements above \(1\) with a \(1\). In other words, for any \(a \in F\):
\[
 \matr{z}'(a) = \begin{cases}
        0, & \text{if } \matr{z}(a) < 0 \\ 1, & \text{if } \matr{z}(a) > 1 \\ \matr{z}(a), & \text{otherwise}
    \end{cases}.
\]
For convenience, denote \(\matr{y} = \begin{pmatrix} \matr{x} \\ \matr{z} \end{pmatrix}\) and \(\matr{y}' = \begin{pmatrix} 
\matr{x}\phantom{'} \\ \matr{z}' \end{pmatrix}\). Observe that the entries of \(\matr{y}\) that lie in the interval \([0, 1]\) are the unchanged in \(\matr{y}'\). Now it suffices to prove:
\begin{gather*}
\left\lVert \matr{W} \matr{B}^\trp \begin{pmatrix} \matr{x\phantom{'}} \\ \matr{z}' \end{pmatrix} \right\rVert_1 \leq \left\lVert \matr{W} \matr{B}^\trp \begin{pmatrix} \matr{x} \\ \matr{z} \end{pmatrix} \right\rVert_1 \\ \Updownarrow \\ \sum_{(a, b) \in E}{w(a, b) \cdot \lvert \matr{y}'(a) - \matr{y}'(b) \rvert} \leq \sum_{(a, b) \in E}{w(a, b) \cdot \lvert \matr{y}(a) - \matr{y}(b) \rvert}.
\end{gather*}
We are going to show the inequality above by showing that, for any edge \((a, b) \in E\), the inequality \(\lvert \matr{y}'(a) - \matr{y}'(b) \rvert \leq \lvert \matr{y}(a) - \matr{y}(b) \rvert\) holds. To this extent, consider fix an edge and perform the following case distinction based on the sets its endpoints belong to:
\begin{enumerate}[I.]
    \item \(a, b \in C\): In this case it holds that \(\matr{y}'(a) = \matr{y}(a) = \matr{x}(a)\) and \(\matr{y}'(b) = \matr{y}(b) = \matr{x}(b)\). Thus, for \(\matr{y}\) both of the endpoints of the edge take values in the interval \([0, 1]\), so the inequality holds trivially.
    \item \(a \in C\), \( b \in F\) or \(a \in F\), \( b \in C\): Without loss of generality, assume that \(a \in C\) and \(b \in F\). This means that \(\matr{y}(a) = \matr{y}'(a) = \matr{x}(a)\), \(\matr{y}(b) = \matr{z}(b)\), and \(\matr{y}'(b) = \matr{z}'(b)\). 
Furthermore, assume that for \(\matr{y}\) one of the endpoints of the edge does not take a value in the interval \([0, 1]\) (otherwise this case would resolve similarly to the previous one), that is, assume that \(\matr{z}(b) \not\in [0, 1]\) holds. Since \(a \in C\), we know that \( \matr{x}(a) \in [0, 1]\).

In order to bound \(\lvert \matr{y}'(a) - \matr{y}'(b) \rvert = \lvert \matr{x}(a) - \matr{z}'(b) \rvert\), we distinguish the following two subcases:
\begin{enumerate}[i.]
    \item \(\matr{z}(b) > 1\): The term can be rewritten as:
    \[
    \lvert \matr{x}(a) - \matr{z}'(b) \rvert = 1 - \matr{x}(a) < \matr{z}(b) - \matr{x}(a) = \lvert \matr{y}(a) - \matr{y}(b) \rvert.
    \]
    \item \(\matr{z}(b) < 0\): The term can be rewritten as:
    \[
    \lvert \matr{x}(a) - \matr{z}'(b) \rvert = \matr{x}(a) - 0 < \matr{x}(a) - \matr{z}(b) = \lvert \matr{y}(a) - \matr{y}(b) \rvert.
    \]
\end{enumerate}
\item \(a, b \in F\): In this case it holds that \(\matr{y}(a) = \matr{z}(a)\), \(\matr{y}'(a) = \matr{z}'(a)\), \(\matr{y}(b) = \matr{z}(b)\), and \(\matr{y}'(b) = \matr{z}'(b)\). Without loss of generality, assume that for \(\matr{y}\) none of the endpoints of the edge take values in the interval \([0, 1]\) (otherwise this case would resolve similarly to one of the previous ones).

In order to bound \(\lvert \matr{y}'(a) - \matr{y}'(b) \rvert = \lvert \matr{z}'(a) - \matr{z}'(b) \rvert\), we distinguish the following two subcases:
\begin{enumerate}[i.]
    \item \(\matr{z}(a) < 0\) and \(\matr{z}(b) < 0\): The term can be rewritten as:
    \[
    \lvert \matr{z}'(a) - \matr{z}'(b) \rvert = \lvert 0 - 0 \rvert = 0 \leq \lvert \matr{z}(a) - \matr{z}(b) \rvert = \lvert \matr{y}(a) - \matr{y}(b) \rvert.
    \]
    \item \(\matr{z}(a) > 1\) and \(\matr{z}(b) > 1\): The term can be rewritten as:
    \[
    \lvert \matr{z}'(a) - \matr{z}'(b) \rvert = \lvert 1 - 1 \rvert = 0 \leq \lvert \matr{z}(a) - \matr{z}(b) \rvert = \lvert \matr{y}(a) - \matr{y}(b) \rvert.
    \]
    \item \(\matr{z}(a) < 0\) and \(\matr{z}(b) > 1\): The term can be rewritten as:
    \[
    \lvert \matr{z}'(a) - \matr{z}'(b) \rvert = \lvert 0 - 1 \rvert = 1 < \lvert \matr{z}(a) - \matr{z}(b) \rvert = \lvert \matr{y}(a) - \matr{y}(b) \rvert.
    \]
    \item \(\matr{z}(a) > 1 \) and \(\matr{z}(b) < 0\): The term can be rewritten as:
    \[
    \lvert \matr{z}'(a) - \matr{z}'(b) \rvert = \lvert 1 - 0 \rvert = 1 < \lvert \matr{z}(a) - \matr{z}(b) \rvert = \lvert \matr{y}(a) - \matr{y}(b) \rvert.
    \]
\end{enumerate}
\end{enumerate}
This concludes the main case distinction, which shows that the program has a minimizer in the set \([0, 1]^F\), since the value attained by \(\matr{z}' \in [0, 1]^F\) is smaller or equal to the one attained by \(\matr{z}\).

\subsection{Proof of Lemma \ref{lemma_program_minimizer_discrete}}
Let \(\matr{z} \in \R^F\) be a minimizer of the program. Note that by Lemma \ref{lemma_program_minimizer_continuous} we can assume \(\matr{z} \in [0, 1]^F\). We will now show that if \(\matr{z}\) has entries that are not in \(\{0, 1\}\), then we can build \(\matr{z}' \in [0, 1]^F\) such that \(\matr{z}'\) is a minimizer as well, and has strictly more entries that are in the set \(\{0, 1\}\). This is enough to prove the lemma, as it shows that one can iteratively reduce the number of entries of \(\matr{z}\) that are not in \(\{0, 1\}\), thus obtaining in the end a minimizer which lies in \(\{0, 1\}^F\).

To that extent let \(r = \min_{a \in F}\{\matr{z}(a) \, | \, \matr{z}(a) > 0\} \) be the value of the smallest non-zero entry of \(\matr{z}\), and \(R = \{a \in V \, | \, \matr{z}(a) = r\} \) the set of nodes that index to that value. The desired \(\matr{z}'\) will be obtained by setting all entries of \(\matr{z}\) that are in \(R\) to \(0\). Now it only remains to prove that \(\matr{z}'\) is a minimizer too.

As an intermediary step towards the proof of the statement above, we show that increasing the values of the entries in \(R\) to \(r + \varepsilon\), as well as decreasing them to \(r - \varepsilon\) still results in a minimizer of the program, where \(\varepsilon > 0\) is sufficiently small such that \(r + \varepsilon\) remains the smallest non-zero value of the vector and \(r - \varepsilon \geq 0\).

Consider thus \(\varepsilon > 0\) with the property above. Furthermore let \( \matr{z}^+_\varepsilon \) be the vector in which all entries of \(\matr{z}\) in \(R\) have been increased to \(r + \varepsilon\), with the rest of the entries being unchanged. We also define \(\matr{z}^-_\varepsilon\) in a similar manner (by decreasing all entries of \(\matr{z}\) in \(R\) to \(r - \varepsilon\)).

For convenience denote \(\matr{y} = \begin{pmatrix} \matr{x} \\ \matr{z} \end{pmatrix} \), \(\matr{y}^+_\varepsilon = \begin{pmatrix} \matr{x} \\ \phantom{^+_\varepsilon}\matr{z}^+_\varepsilon \end{pmatrix} \), and \(\matr{y}^-_\varepsilon = \begin{pmatrix} \matr{x} \\ \phantom{^-_\varepsilon}\matr{z}^-_\varepsilon \end{pmatrix} \). Without loss of generality, assume henceforth that the edges in \(E\) is directed  such that they point to the node with the greater value in \(\matr{y}\), that is \(\matr{y}(a) \leq \matr{y}(b)\) for all \((a, b) \in E\). Note that by the way we defined \(\varepsilon\), it also follows that \(\matr{y}^+_\varepsilon(a) \leq \matr{y}^+_\varepsilon(b)\) and \(\matr{y}^-_\varepsilon(a) \leq \matr{y}^-_\varepsilon(b)\) for all \((a, b) \in E\).

Recall that our current aim is to show that both \(\matr{z}^+_\varepsilon\) and \(\matr{z}^-_\varepsilon\) still are minimizers of the program. This will be achieved by inspecting how the terms of the sum
\[
 \left\lVert \matr{W} \matr{B}^\trp \begin{pmatrix} \matr{x} \\ \matr{z} \end{pmatrix} \right\rVert_1 = \left\lVert \matr{W} \matr{B}^\trp \matr{y} \right\rVert_1 = \sum_{(a, b) \in E}{w(a, b) \cdot (\matr{y}(b) - \matr{y}(a))}
\]
change when \(\matr{z}\) gets replaced by \(\matr{z}^+_\varepsilon\), and \(\matr{z}^-_\varepsilon\) respectively.

%\begin{comment}
Observe that a term in the sum above corresponding to the edge \((a, b) \in E \) changes if and only if exactly one of \(a\) and \(b\) is in \(R\) (otherwise the term does not change, since entries outside of \(R\) retain the same value, and entries in \(R\) change by the same amount, namely \(\varepsilon\)). Taking into account our assumption about the orientation of the edges, let \(E', E'' \subseteq E\) be the following:
\begin{align*}
E' &= \{(a, b) \in E \, | \, \matr{y}(a) = 0, \, \matr{y}(b) = r\} \\
E'' &= \{(a, b) \in E \, | \, \matr{y}(a) = r, \, \matr{y}(b) > r\}.
\end{align*}

Since \(r\) is the smallest non-zero value of \(\matr{z}\), and \(\varepsilon\) has been chosen to be sufficiently small, we can write out the values of the program for \(\matr{z}^+_\varepsilon\) and \(\matr{z}^-_\varepsilon\) as follows:
\begin{equation}
\begin{aligned}
\label{equation_program_yp_ym}
\left\lVert \matr{W} \matr{B}^\trp \matr{y}^+_\varepsilon \right\rVert_1 &= \sum_{(a, b) \in E'}{w(a, b) \cdot (\matr{y}^+_\varepsilon(b) - \matr{y}^+_\varepsilon(a))}\\ &+ \sum_{(a, b) \in E''}{w(a, b) \cdot (\matr{y}^+_\varepsilon(b) - \matr{y}^+_\varepsilon(a))}\\ & + \sum_{(a, b) \in E \setminus (E' \cup E'')}{w(a, b) \cdot (\matr{y}^+_\varepsilon(b) - \matr{y}^+_\varepsilon(a))}\\
& = \sum_{(a, b) \in E'}{w(a, b) \cdot (r + \varepsilon)} + \sum_{(a, b) \in E''}{w(a, b) \cdot (\matr{y}(b) - r - \varepsilon)} \\ & + \sum_{(a, b) \in E \setminus (E' \cup E'')}{w(a, b) \cdot (\matr{y}(b) - \matr{y}(a))}, \\
\left\lVert \matr{W} \matr{B}^\trp \matr{y}^-_\varepsilon \right\rVert_1 &= \sum_{(a, b) \in E'}{w(a, b) \cdot (\matr{y}^-_\varepsilon(b) - \matr{y}^-_\varepsilon(a))}\\ &+ \sum_{(a, b) \in E''}{w(a, b) \cdot (\matr{y}^-_\varepsilon(b) - \matr{y}^-_\varepsilon(a))}\\ & + \sum_{(a, b) \in E \setminus (E' \cup E'')}{w(a, b) \cdot (\matr{y}^-_\varepsilon(b) - \matr{y}^-_\varepsilon(a))}\\
& = \sum_{(a, b) \in E'}{w(a, b) \cdot (r - \varepsilon)} + \sum_{(a, b) \in E''}{w(a, b) \cdot (\matr{y}(b) - r + \varepsilon)} \\ & + \sum_{(a, b) \in E \setminus (E' \cup E'')}{w(a, b) \cdot (\matr{y}(b) - \matr{y}(a))}.
\end{aligned}
\end{equation}
%\end{comment}
Note that the value of the program for \(\matr{z}\) can be rewritten as:
\begin{equation}
\begin{aligned}
\label{equation_program_value_expl}
\left\lVert \matr{W} \matr{B}^\trp \matr{y} \right\rVert_1 &= \sum_{(a, b) \in E'}{w(a, b) \cdot r} + \sum_{(a, b) \in E''}{w(a, b) \cdot (\matr{y}(b) - r)} \\ & + \sum_{(a, b) \in E \setminus (E' \cup E'')}{w(a, b) \cdot (\matr{y}(b) - \matr{y}(a))}.
\end{aligned}
\end{equation}
Recall that \(\matr{z}\) is a minimizer for the program, which implies:
\[
\left\lVert \matr{W} \matr{B}^\trp \matr{y} \right\rVert_1 \leq \left\lVert \matr{W} \matr{B}^\trp \matr{y}^+_\varepsilon \right\rVert_1 \text{ and } \left\lVert \matr{W} \matr{B}^\trp \matr{y} \right\rVert_1 \leq \left\lVert \matr{W} \matr{B}^\trp \matr{y}^-_\varepsilon \right\rVert_1.
\]
We can then simplify the previous inequalities by using Equations \eqref{equation_program_value_expl} and \eqref{equation_program_yp_ym}, yielding:

\begin{gather*}
0 \leq \sum_{(a, b) \in E'}{w(a, b)} - \sum_{(a, b) \in E''}{w(a, b)} \text{ and } 0 \leq \sum_{(a, b) \in E''}{w(a, b)} - \sum_{(a, b) \in E'}{w(a, b)} \\ \Updownarrow \\ \sum_{(a, b) \in E'}{w(a, b)} = \sum_{(a, b) \in E''}{w(a, b)}.
\end{gather*}

This essentially means that if we vary the values of the entries in \(R\) by a quantity \(\delta\) in an interval that preserves the relative order of the entries, the value of the resulting program will describe a linear function with respect to \(\delta\) for that interval. And since a minimum of this function lies by assumption strictly inside the interval, this function has to be constant on that interval. Hence, choosing a \(\delta = -r\) (note that \(-r\) is a viable choice, as we assumed \(r\) to be the smallest non-zero value of \(\matr{z}\)) will ``shift'' all the values of entries in \(R\) to \(0\), and yield the desired \(\matr{z}'\), while still resulting in a minimizer of the program.

Thus, we have shown that starting from a minimizer in \([0, 1]^F \setminus \{0, 1\}^F\) it is possible to construct one with strictly more entries in the set \(\{0, 1\}\), which effectively proves the lemma.

\subsection{Proof of Lemma \ref{lemma_energy_minimizer_in_01}}

The proof of this lemma is very similar to the one of Lemma \ref{lemma_program_minimizer_continuous}. We will write out the first part in detail, but since the second part of the proof proceeds with an analogous case distinction, we refer to the corresponding section of the proof of Lemma \ref{lemma_program_minimizer_continuous} for completeness.

We prove this lemma by showing that from any \(\matr{y} \in \R^F\) we can construct \(\matr{y}' \in [0, 1]^F\), such that the value for \(\matr{y}'\) of the given program is less or equal to the one for \(\matr{y}\). Therefore, there will always exist a minimizer of the program that lies in \([0, 1]^F\).

Thus, for a fixed \(\matr{x} \in [0, 1]^C\), let \(\matr{y} \in \R^F\) be arbitrary and construct \(\matr{y}'\) by ``capping'' all elements of \(\matr{y}\) below \(0\) with a \(0\) in that respective entry, and all elements above \(1\) with a \(1\). In other words, for any \(a \in F\):
\[
 \matr{y}'(a) = \begin{cases}
        0, & \text{if } \matr{y}(a) < 0 \\ 1, & \text{if } \matr{y}(a) > 1 \\ \matr{y}(a), & \text{otherwise}
    \end{cases}.
\]
For convenience, denote \(\matr{v} = \begin{pmatrix} \matr{x} \\ \matr{y} \end{pmatrix}\) and \(\matr{v}' = \begin{pmatrix} 
\matr{x}\phantom{'} \\ \matr{y}' \end{pmatrix}\). Observe that the entries of \(\matr{v}\) that lie in the interval \([0, 1]\) are the unchanged in \(\matr{v}'\). Now it suffices to prove:
\begin{gather*}
\begin{pmatrix} \matr{x} \\ \phantom{'} \matr{y}' \end{pmatrix}^\trp \matr{L} \begin{pmatrix} \matr{x} \\ \phantom{'} \matr{y}' \end{pmatrix} \leq \begin{pmatrix} \matr{x} \\ \matr{y} \end{pmatrix}^\trp \matr{L} \begin{pmatrix} \matr{x} \\ \matr{y} \end{pmatrix} \\ \Updownarrow \\ \sum_{(a, b) \in E}{w(a, b) \cdot \left(\matr{v}'(a) - \matr{v}'(b)\right)^2} \leq \sum_{(a, b) \in E}{w(a, b) \cdot (\matr{v}(a) - \matr{v}(b))^2}.
\end{gather*}
We are going to show the inequality above by showing that, for any edge \((a, b) \in E\), the inequality \(\left( \matr{v}'(a) - \matr{v}'(b) \right)^2 \leq (\matr{v}(a) - \matr{v}(b))^2\) holds.

Note that at this point, showing \(\left( \matr{v}'(a) - \matr{v}'(b) \right)^2 \leq (\matr{v}(a) - \matr{v}(b))^2\) is equivalent to proving \(\left\lvert \matr{v}'(a) - \matr{v}'(b) \right\rvert \leq \lvert \matr{v}(a) - \matr{v}(b) \rvert \). The case distinction that would conclude this proof has been already carried out in detail in the proof of Lemma \ref{lemma_program_minimizer_continuous} (and in a slightly more general setting).
